# Supplementary material for: Sampling weights of deep neural networks
Source: arXiv:2306.16830 source file (2023-11-12)
Supplement: Supplementary file 1 [file numerical_experiments_overview.tex]

\section{Numerical experiments} \label{appendix:numerical_experiments}
\tabref{tab:hyperparameters} contains an overview of the most important hyper-parameters used in the numerical experiments.
\begin{table}[]
    \caption{Hyper-parameters for the numerical experiments in the paper.}\label{tab:hyperparameters}\centering
\begin{tabularx}{\textwidth}{XXXX}
    \textbf{Name} & \textbf{\#layers} & \textbf{\#Neurons} & \textbf{Regularization}\\
    Illustration;\secref{appendix:barron_illustration} & 1-3 & 64--8096 & 1E-10
\end{tabularx}
\end{table}
